# Supplementary material for: Optimal inference for the mean of random functions
Source: arXiv:2504.11025 source file (2025-04-15)
Supplement: Supplementary file 1 [file SM_sum_sin_cos.tex]

% !TeX root = ../mean_SM.tex

%%%%%%%%%%%%%%%%%%%%%%%%%%
%%%%%%%%%%%%%%%%%%%%%%%%%%
%%%%%%%%%%%%%%%%%%%%%%%%%%
%%%%%%%%%%%%%%%%%%%%%%%%%% The working version as created by Valentin Jan 12
%%%%%%%%%%%%%%%%%%%%%%%%%%

\begin{lemma}\label{sum_sin_cos}
	For $\mathbf t \in \mathcal T$ and $L\in \mathbb N$, let
	$$\theta (L, D)= \sum_{ | \mathbf k|_1 \leq 2L } \phi_{\mathbf k} ^2(\mathbf t).$$ 
	Then, for any $\mathbf t \in \mathcal T$, we have 
	\begin{equation}
		\frac{1}{L} \sum_{j=0}^{L-1}\theta (L+j, D) = \frac{2^{2D+1} -2^D}{ (D+1)!} L^D + O(L^{D-1}) = \frac{2^{2D+1} -2^D}{ (D+1)!} L^D\{1+o(1)\},
	\end{equation}
	and the constants in the terms $O(L^{D-1})$ and $o(1)$ do not depend on $\mathbf t$.
\end{lemma}

\medskip

\begin{proof}[Proof of Lemma \ref{sum_sin_cos}]
	Let $J \in \mathbb N$, we have 
	\begin{multline}
		\theta (J, D)=\sum_{ | \mathbf k|_1 \leq 2J } \phi_{\mathbf k} ^2(\mathbf t) = 1 + \sum_{\ell=1}^{ 2J} \sum_{ \{k_1+ k_2 + \dots + k_D = \ell\}}\prod _{j=1}^D \phi_{ k_j} ^2(t_j)\\
			= 1 + \sum_{\ell=1}^{ J}\left\{ \sum_{ k_1= 0}^{ 2\ell}\sum_{ \{ k_2 + \dots + k_D = 2\ell -k_1\}}\prod _{j=1}^D \phi_{ k_j} ^2(t_j) +  \sum_{ k_1= 0}^{ 2\ell- 1}\sum_{  \{k_2 + \dots + k_D = (2\ell -1) -k_1\}}\prod _{j=1}^D \phi_{ k_j} ^2(t_j)\right\}\\
		\hspace{-7.6cm}= 1 + \underbrace{\sum_{\ell=1}^{ 2J} \sum_{  \{k_2 + \dots + k_D = \ell\}}\prod _{j=2}^D \phi_{ k_j} ^2(t_j)}_{\beta(J,D-1)}\\
			\quad \quad + \sum_{\ell=1}^{ J} \left\{\sum_{ k_1= 1}^{ 2\ell}\sum_{ \{ k_2 + \dots + k_D = 2\ell -k_1\}}\prod _{j=1}^D \phi_{ k_j} ^2(t_j) +  \sum_{ k_1= 1}^{ 2\ell- 1}\sum_{  \{k_2 + \dots + k_D = (2\ell -1) -k_1\}}\prod _{j=1}^D \phi_{ k_j} ^2(t_j)\right\}\\
		\hspace{-10.7cm} = : 1 + \beta (J, D-1)
		%\sum_{\ell=1}^{ 2J} \sum_{  k_2 + \dots + k_D = \ell}\prod _{i=2}^D \phi_{ k_j} ^2(t_j)
		\\
		+ \sum_{\ell=1}^{ J} \sum_{ k_1=1}^{ \ell}\left\{\sum_{\{  k_2 + \dots + k_D = 2\ell -2k_1\}} \phi_{2k_1}^2(t_1) \prod _{j=2}^D \phi_{ k_j} ^2(t_j)\right.\\ \hspace{4.2cm}\left. + \sum_{  \{k_2 + \dots + k_D = 2\ell -(2k_1-1)\}} \phi_{2k_1 -1}^2(t_1)\prod _{j=2}^D \phi_{ k_j} ^2(t_j)\right\} \\
		+  \sum_{\ell=1}^{ J}\left\{ \sum_{ k_1= 1}^{ \ell-1}\sum_{  \{k_2 + \dots + k_D = (2\ell -1) -2k_1\}} \phi_{2k_1}^2(t_1)\prod _{j=2}^D \phi_{ k_j} ^2(t_j) \right.\\ \hspace{6cm}\left. +\sum_{ k_1= 1}^{ \ell}\sum_{ \{ k_2 + \dots + k_D = (2\ell-1)  -(2k_1-1)\}} \phi_{2k_1-1}^2(t_1)\prod _{j=2}^D \phi_{ k_j} ^2(t_j)\right\}	.	
	\end{multline}		
Grouping terms and using the fact that $\phi_{2k_1-1}^2(t_1)+\phi_{2k_1}^2(t_1)=2$, 
we get		
		\begin{multline}	
		\theta (J, D)= 1 
		%+\sum_{\ell=1}^{ 2J} \sum_{  k_2 + \dots + k_D = \ell}\prod _{i=2}^D \phi_{ k_j} ^2(t_j)
		+\beta (J, D-1)
		+2\sum_{\ell=1}^{ J} \sum_{ k_1= 1}^{ \ell}\sum_{\{  k_2 + \dots + k_D = 2\ell -2k_1\}}\prod _{j=2}^D \phi_{ k_j} ^2(t_j) \\
		+\sum_{\ell=1}^{ J}  \left\{\sum_{ k_1= 1}^{ \ell-1}\sum_{  \{k_2 + \dots + k_D = 2\ell-2k_1-1\}} \phi_{2k_1}^2(t_1)\prod _{i=2}^D \phi_{ k_j} ^2(t_j)\right.\\ \hspace{8cm}\left.+\sum_{ k_1= 1}^{ \ell}\sum_{  \{k_2 + \dots + k_D = 2\ell -2k_1+1\}} \phi_{2k_1-1}^2(t_1)\prod _{i=2}^D \phi_{ k_j} ^2(t_j)\right\}\\
		=: 1	+\beta (J, D-1)+ 		2\sum_{\ell=1}^{ J} \sum_{ k_1= 1}^{ \ell}\sum_{\{  k_2 + \dots + k_D = 2\ell -2k_1\}}\prod _{j=2}^D \phi_{ k_j} ^2(t_j) + S(J).
	\end{multline}
	Using Fubini for the last sums, we can write,	
	\begin{multline}
	%	\sum_{\ell=1}^{ J}  \left\{\sum_{ k_1= 1}^{ \ell-1}\sum_{  \{k_2 + \dots + k_D = 2\ell -2k_1-1\}} \phi_{2k_1}^2(t_1)\prod _{j=2}^D \phi_{ k_j} ^2(t_j)\right.\\ \hspace{4cm}\left. +\sum_{ k_1= 1}^{ \ell}\sum_{  \{k_2 + \dots + k_D = 2\ell -2k_1+1\}} \phi_{2k_1-1}^2(t_1)\prod _{j=2}^D \phi_{ k_j} ^2(t_j)\right\}\\
	S(J)	= \sum_{k_1= 1}^{J-1}\sum_{\ell=k_1+1 }^J\sum_{  \{k_2 + \dots + k_D = 2\ell -2k_1-1\}} \phi_{2k_1}^2(t_1)\prod _{j=2}^D \phi_{ k_j} ^2(t_j) \\
			\hspace{4cm}+ \sum_{k_1= 1}^{J} \sum_{\ell=k_1 }^J\sum_{  \{k_2 + \dots + k_D = 2\ell -2k_1+1\}} \phi_{2k_1-1}^2(t_1)\prod _{j=2}^D \phi_{ k_j} ^2(t_j)\\
	\stackrel{\ell^\prime = \ell+1}{=}	 \sum_{k_1= 1}^{J-1}\sum_{\ell^\prime=k_1 }^{J-1}\sum_{  \{k_2 + \dots + k_D = 2\ell^\prime  -2k_1+1\}} \phi_{2k_1}^2(t_1)\prod _{j=2}^D \phi_{ k_j} ^2(t_j) \\
		\hspace{4cm}+ \sum_{k_1= 1}^{J} \sum_{\ell=k_1 }^J\sum_{  \{k_2 + \dots + k_D = 2\ell -2k_1+1\}} \phi_{2k_1-1}^2(t_1)\prod _{j=2}^D \phi_{ k_j} ^2(t_j)\\
		= \sum_{k_1= 1}^{J-1}\sum_{\ell^\prime=k_1 }^{J-1}\sum_{  \{k_2 + \dots + k_D = 2\ell^\prime +1 -2k_1\}} \phi_{2k_1}^2(t_1)\prod _{j=2}^D \phi_{ k_j} ^2(t_j) \\
		\hspace{4cm}+ \sum_{k_1= 1}^{J-1} \sum_{\ell=k_1 }^{J-1}\sum_{  \{k_2 + \dots + k_D = 2\ell -2k_1+1\}} \phi_{2k_1-1}^2(t_1)\prod _{j=2}^D \phi_{ k_j} ^2(t_j)\\
		\hspace{5cm}+ \sum_{k_1= 1}^{J} \sum_{  \{k_2 + \dots + k_D = 2J -2k_1+1\}} \phi_{2k_1-1}^2(t_1)\prod _{j=2}^D \phi_{ k_j} ^2(t_j) \\
	\stackrel{\phi_{2k_1-1}^2(t_1)+\phi_{2k_1}^2(t_1)=2}{=}2 \sum_{k_1= 1}^{J-1} \sum_{\ell=k_1 }^{J-1}\sum_{  \{k_2 + \dots + k_D = 2\ell -2k_1+1\}} \prod _{j=2}^D \phi_{ k_j} ^2(t_j)\\
		\hspace{4cm}+ \sum_{k_1= 1}^{J} \sum_{  \{k_2 + \dots + k_D = 2J -2k_1+1\}} \phi_{2k_1-1}^2(t_1)\prod _{j=2}^D \phi_{ k_j} ^2(t_j).
	\end{multline}
	Therefore, using again Fubini, the fact that $\phi_{2k_1-1}^2(t_1)=2- \phi_{2k_1}^2(t_1)$, we get
	\begin{multline}
		\theta (J, D ) 
		%\sum_{ | \mathbf k|_1 \leq 2J } \phi_{\mathbf k} ^2(\mathbf t) 
		=1 +  \beta (J, D-1)
	%	\\+\sum_{\ell=1}^{ 2J} \sum_{  k_2 + \dots + k_D = \ell}\prod _{j=2}^D \phi_{ k_j} ^2(t_j)
			\\+2\left\{\sum_{\ell=1}^{ J} \sum_{ k_1= 1}^{ \ell}\sum_{\{  k_2 + \dots + k_D = 2\ell -2k_1\}}\prod _{j=2}^D \phi_{ k_j} ^2(t_j) 
			+\sum_{k_1= 1}^{J-1} \sum_{\ell=k_1 }^{J-1}\sum_{  \{k_2 + \dots + k_D = 2\ell -2k_1+1\}} \prod _{j=2}^D \phi_{ k_j} ^2(t_j)\right\}
		\\+ \sum_{k_1= 1}^{J} \sum_{  \{k_2 + \dots + k_D = 2J -2k_1+1\}} \phi_{2k_1-1}^2(t_1)\prod _{j=2}^D \phi_{ k_j} ^2(t_j)\\
		\hspace{-9.2cm}= 1 + \beta (J, D-1)
		%\sum_{\ell=1}^{ 2J} \sum_{  k_2 + \dots + k_D = \ell}\prod _{j=2}^D \phi_{ k_j} ^2(t_j)
		\\	+2\left\{\sum_{\ell=1}^{ J} \sum_{ k_1= 1}^{ \ell}\sum_{\{  k_2 + \dots + k_D = 2\ell -2k_1\}}\prod _{j=2}^D \phi_{ k_j} ^2(t_j) 
			+\sum_{\ell= 1}^{J} \sum_{k_1=1 }^{\ell}\sum_{  \{k_2 + \dots + k_D = 2\ell -2k_1+1\}} \prod _{j=2}^D \phi_{ k_j} ^2(t_j)\right\}
		\\+ \sum_{k_1= 1}^{J} \sum_{  \{k_2 + \dots + k_D = 2J -2k_1+1\}} (\phi_{2k_1-1}^2(t_1)-2)\prod _{j=2}^D \phi_{ k_j} ^2(t_j)\\
		=1+\beta (J, D-1)
	%	\underbrace{1 + \sum_{\ell=1}^{ 2J} \sum_{  k_2 + \dots + k_D = \ell}\prod _{j=2}^D \phi_{ k_j} ^2(t_j)}_{=O(J^{D-1})}
		+2\sum_{\ell=1}^{ J} \sum_{ k_1= 1}^{2 \ell}\sum_{\{  k_2 + \dots + k_D = 2\ell -k_1\}}\prod _{j=2}^D \phi_{ k_j} ^2(t_j) \\
		- \underbrace{\sum_{k_1= 1}^{J} \sum_{  \{k_2 + \dots + k_D = 2J -2k_1+1\}} \phi_{2k_1}^2(t_1)\prod _{j=2}^D \phi_{ k_j} ^2(t_j)}_{=\gamma(J,D-1)}\\
		= 1+\beta (J, D-1)  + 2\sum_{\ell=1}^J \{\theta(\ell, D-1)- \delta(D-1)\} - \gamma(J,D-1),
	\end{multline}
	where 
	$$
	\delta(\ell, D-1) = \sum_{\{  k_2 + \dots + k_D = 2\ell  \}}\prod _{j=2}^D \phi_{ k_j} ^2(t_j)\lesssim \ell^{D-2},
	$$
		with the constant in $\lesssim$ depending only on $D$.
	Moreover, it is easy to notice that
	$$
\max\{ \beta (J, D-1),	\gamma(J,D-1), \theta(0, D-1)\}\lesssim J ^{D-1},
	$$
	with the constant in $\lesssim$ depending only on $D$.
	Therefore, we have 
	\begin{equation}
		\theta(J,D)= 2\sum_{\ell=0}^J \theta(\ell, D-1) + O(J^{D-1})= \left\{2\sum_{k_1=0}^J2 \sum_{k_2=0}^{k_1}\dots 2\sum_{k_D=0}^{k_{D-1}} 1\right\}+ O(J^{D-1}) .
	\end{equation}
	Faulhaber's formula, see \citet[ page 106]{Conway96}, gives  the coefficient of the largest power in the sum of positive powers. Thus
	\begin{equation}
		\theta(J,D)= \frac{2^{D}}{D!} J^D + O(J^{D-1}).
	\end{equation}
	The constant in the term $O(J^{D-1})$ does not depend on $\mathbf t$. 
	Thus, using Faulhaber's formula again, we get 
	\begin{multline}
		\frac{1}{L} \sum_{j=0}^{L-1}\theta (L+j, D) = \frac{2^{D}}{D! L}\sum_{j=0}^{L-1} (L+j)^D + O(L^{D-1})
	\\	= \frac{2^{D}}{D! L}\sum_{j=0}^{L-1}\sum_{k=0}^D \binom{D}{k} j^k L^{D-k} + O(L^{D-1})\\
		=  \frac{2^{D}}{D! L}\sum_{k=0}^D\binom{D}{k}  L^{D-k}\sum_{j=0}^{L-1} j^k + O(L^{D-1})
		\\\qquad = \frac{2^{D}}{D! L}\sum_{k=0}^D\frac{1}{k+1}\binom{D}{k}  L^{D-k}L^{k+1}+ O(L^{D-1})\\
		\quad =\frac{2^{D}}{D! }L^D \sum_{k=0}^D\frac{1}{D+1}\binom{D+1}{k+1}+ O(L^{D-1})
		\\=\frac{2^{D} ( 2^{D+1} -1)}{D!(D+1) }L^D + O(L^{D-1}).
	\end{multline}
	The constant in $O(L^{D-1})$ does not depend on $\mathbf t$. The proof  is now complete. \end{proof}
