# Supplementary material for: Optimal inference for the mean of random functions
Source: arXiv:2504.11025 source file (2025-04-15)
Supplement: Supplementary file 2 [file subsampling_SM.tex]

% !TeX root = ../mean_SM.tex

\subsection{Finite sample confidence regions by subsampling}\label{subssampl_SM}

To construct confidence regions without estimating the matrix $\Sigma$, we use a subsampling method that involves estimating the mean function using subsamples of the original dataset. This is an ensemble method, akin to the technique used for example  in Bagging; see \cite{buhlmann2012bagging} and \cite{buja2006observations}.  For any set $\mathcal S$, let $|\mathcal S|$ denote its cardinal. 
%Theoretical aspects of subsampling are discussed in \cite{politis1994} and related works.

Formally, let $\mathcal{E}^{\rm obs} = \{(i,m) : 1 \leq m \leq M_i, 1 \leq i \leq N\}$ denote the set of observed data indices. For a subset $\mathcal{A} \subset \mathcal{E}^{\rm obs}$, let $\widehat{\mu}^*(\cdot, \mathcal{A})$ be the estimated mean function constructed with the data $\{(Y_{i,m}, \mathbf{T}_{i,m}) : (i,m)  \in \mathcal{A}\}$ and the $L^*$ defined as in \eqref{L_general} with $|\mathcal A|$ instead of  $\overline M$ .
Furthermore, we denote by  $\mathcal{A}^{\rm subj}$ the subset of indices of the random functions with design points selected in the subsample $\mathcal{A}$  that is  $\mathcal{A}^{\rm subj} = \{1\leq i \leq N : \exists m \in \mathbb{N}^*, (i,m) \in \mathcal{A}\}$.
Moreover, for   $ i \in \mathcal A^{\rm subj}$, let $ \mathcal A^{\rm obj}(i)= \{ m\in \mathbb N^*: (i,m) \in \mathcal A\}$. We also define
$$
\Delta (\mathbf t, \mathcal{A}) =  \widehat{\mu}^{*}(\mathbf t, \mathcal A) -  \widehat{\mu}^{*}(\mathbf t)  , \qquad \Delta_{\infty}(\mathcal{A}) = %\sup_{\mathbf t \in \mathcal{T}} 
\left\| \widehat{\mu}^{*}(\cdot, \mathcal{A}) - \widehat{\mu}^{*}(\cdot)  \right\|_\infty,  
$$
and, for $\vartheta(|\mathcal A|) \geq 1$, let
$$
\tau_{\mathcal{A}} =\left(\vartheta(|\mathcal A|)  |\mathcal A|^{\frac{ \alphamu}{2\alphamu+D}}\right) \wedge \frac{ \sum_{ i \in \mathcal{A}^{\rm subj}} |\mathcal A^{\rm obj}(i)| }{  \sqrt{\sum_{ i \in \mathcal{A}^{\rm subj}} |\mathcal A^{\rm obj}(i)| (|\mathcal A^{\rm obj}(i)|  - 1)}}.
$$
By construction, $\tau_{\mathcal{E}^{obs}}$ is equal to $\min\{\vartheta(\overline M )r_1(L^*),r_2\}$ considered
in Corollary  \ref{coro_CB2}. Let $\mathcal{U}(z, \mathbf{t})$ and $\mathcal{U}_{\infty}(z)$ be the (non-asymptotic) CDFs of $\tau_{\mathcal{E}^{obs}} \Delta(\mathbf{t})$ and $\tau_{\mathcal{E}^{obs}} \Delta_{\infty}$, respectively. For  $\alpha \in (0,1)$, let
\begin{equation}
	c_N(\mathbf t, 1 - \alpha) = \inf\{ z : \mathcal{U}( z, \mathbf t) \geq 1 - \alpha\}, \qquad c_{N, \infty}(1 - \alpha) = \inf\{ z : \mathcal{U}_\infty( z) \geq 1 - \alpha\},
\end{equation}
be the associated  $(1 - \alpha)-$quantiles.
These CDFs and their quantiles can be approximated by subsampling. 

Following the findings in \cite{buja2006observations}, we consider subsamples $\mathcal A$ with  $|\mathcal A|=\lfloor \overline{M} / 2 \rfloor$. Let $N_s$ be the number of subsamples $\mathcal A$. For a fixed $z \in \mathbb{R}_+$, we uniformly draw $N_s$ subsets $\mathcal{A}_1, \dots, \mathcal{A}_{N_s} \subset \mathcal{E}^{obs}$ of size $\lfloor \overline{M} / 2 \rfloor$, and define:
\begin{equation}
	\widetilde {\mathcal U}( z,\mathbf  t) = \frac{1}{N_s} \sum_{1 \leq j \leq N_s} \mathbbm{1} \{\tau_{\mathcal{A}_j} \Delta(\mathbf t, \mathcal{A}_j) \leq z\} , \qquad \widetilde {\mathcal U}_\infty (z) = \frac{1}{N_s} \sum_{1 \leq j \leq N_s} \mathbbm{1}\{\tau_{\mathcal{A}_j} \Delta_\infty( \mathcal{A}_j) \leq z\} .
\end{equation}
For the theory it suffices to take $N_s = a N$ with some $a>0$. Note that the condition $\min \{r_1(L^*), r_2\}\rightarrow \infty$  implies $\tau_{\mathcal{A}}, N_s\rightarrow \infty$.  The estimated quantiles are then
\begin{equation}
	\widetilde c(\mathbf t, 1 - \alpha) = \inf\{ z :\widetilde  {\mathcal{U}}( z, \mathbf t) \geq 1 - \alpha\}, \qquad \widetilde  c_{\infty}(1 - \alpha) = \inf\{ z :\widetilde { \mathcal{U}}_\infty( z) \geq 1 - \alpha\}.
\end{equation}
Then, for any $\mathbf t \in \mathcal T$, our  pointwise confidence interval of level $(1-\alpha)$ is  
$$
CI(\mathbf t)=[\widehat{\mu}^{*}(\mathbf t) -\widetilde c(\mathbf t , 1 - \alpha/2)/ \tau_{\mathcal E^{obs}}\;,\;   \widehat{\mu}^{*}(\mathbf t)  -\widetilde c(\mathbf t, \alpha/2)/ \tau_{\mathcal E^{obs}} ].
$$
Moreover, the  uniform confidence band is given by the following lower and upper limits~:
$$
L(\mathbf t) = \widehat{\mu}^{*}(\mathbf t) -\widetilde  c_{ \infty}(1 - \alpha)/ \tau_{\mathcal E^{obs}}\quad \text{and} \quad U(\mathbf t) = \widehat{\mu}^{*}(\mathbf t) +\widetilde  c_{ \infty}(1 - \alpha)/ \tau_{\mathcal E^{obs}},\qquad \mathbf t \in\mathcal T.
$$
We adopt the notation from \cite{CBadapt2014} and write $CB=[L(\mathbf t), U(\mathbf t)]$. 
In view of the non-asymptotic Gaussian approximation result in Theorem \ref{normal_approximation}, and the Corollaries \ref{coro_linear} and \ref{coro_CB}, below we conjecture the validity of our confidence sets. 
%The proof is omitted. 

\medskip

\begin{conjecture}\label{cor_sub_samp}
	Assume that the conditions of Corollary \ref{coro_CB2} hold true, and $N_s = aN$ for some $a>0$. Then, for any $\mathbf{t}\in \mathcal{T} $,  if $\vartheta(\overline M) \rightarrow \infty$ or $r_2 \ll r_1(L^*)$, we have
	\begin{equation}
		\mathbb{P} \big( \mu( \mathbf{t}) \in CI(\mathbf{t}) \big)\rightarrow  1-\alpha
		\qquad \text{ and } \qquad 
		\mathbb{P} \big( \mu( \mathbf{s}) \in CB, \; \forall \mathbf{s} \in \mathcal{T} \big)\rightarrow 1-\alpha.
	\end{equation}
	If $\vartheta(\overline M) =1$ and $r_1(L^*)\lesssim r_2$, we conjecture that the  result remains true with $V_{L^*}(\mu;\cdot) $ replacing $\mu(\cdot)$.
\end{conjecture}
